# Supplementary material for: Enhanced Microfluidic Mixing via a Tricritical Spiral Vortex Instability
Source: arXiv:1509.00951 source file (2015-09-03)
Supplement: Supplementary file 1 [file Supplementary_Figures_comp.pdf]

**Enhanced Microfluidic Mixing via a Tricritical Spiral Vortex Instability**

*S. J. Haward, R. J. Poole, M. A. Alves, P. J. Oliveira, N. Goldenfeld, A. Q. Shen*

## ELECTRONIC SUPPLEMENTARY FIGURES

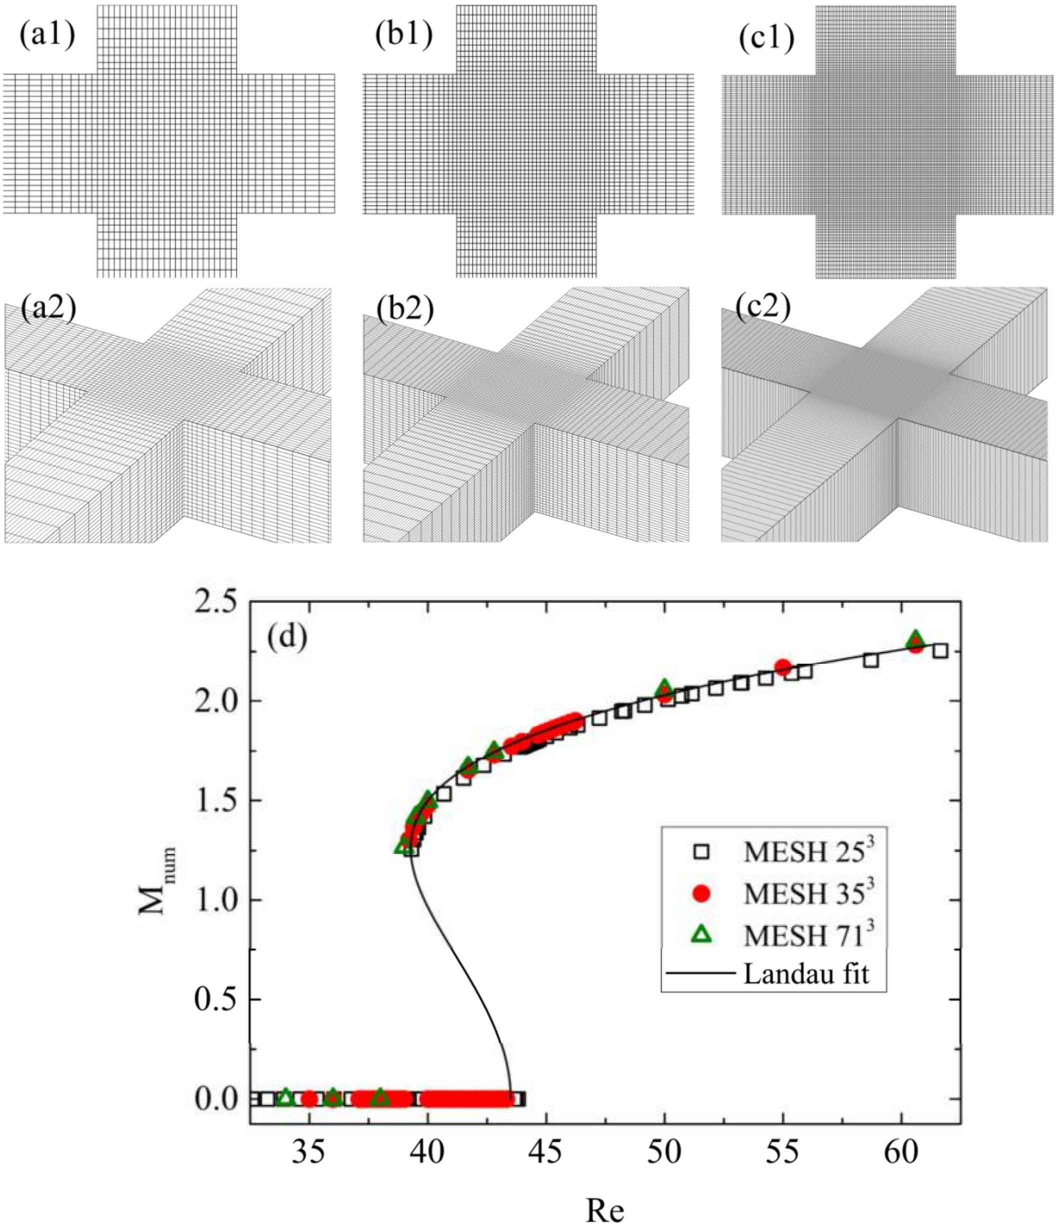


**FIG S1**: (a1) – (c1) top down views, and (a2) – (c2) 3D views for channel $\alpha = 1$ of the numerical meshes employed in the flow simulations: (a) $25^3$, (b) $35^3$, and (c) $71^3$ control volumes. Comparison between the simulation results with the various meshes in the channel with $\alpha = 1$, fitted with the Landau $6^{th}$ order polynomial potential (Eqs. (3 – 5) in the main text).

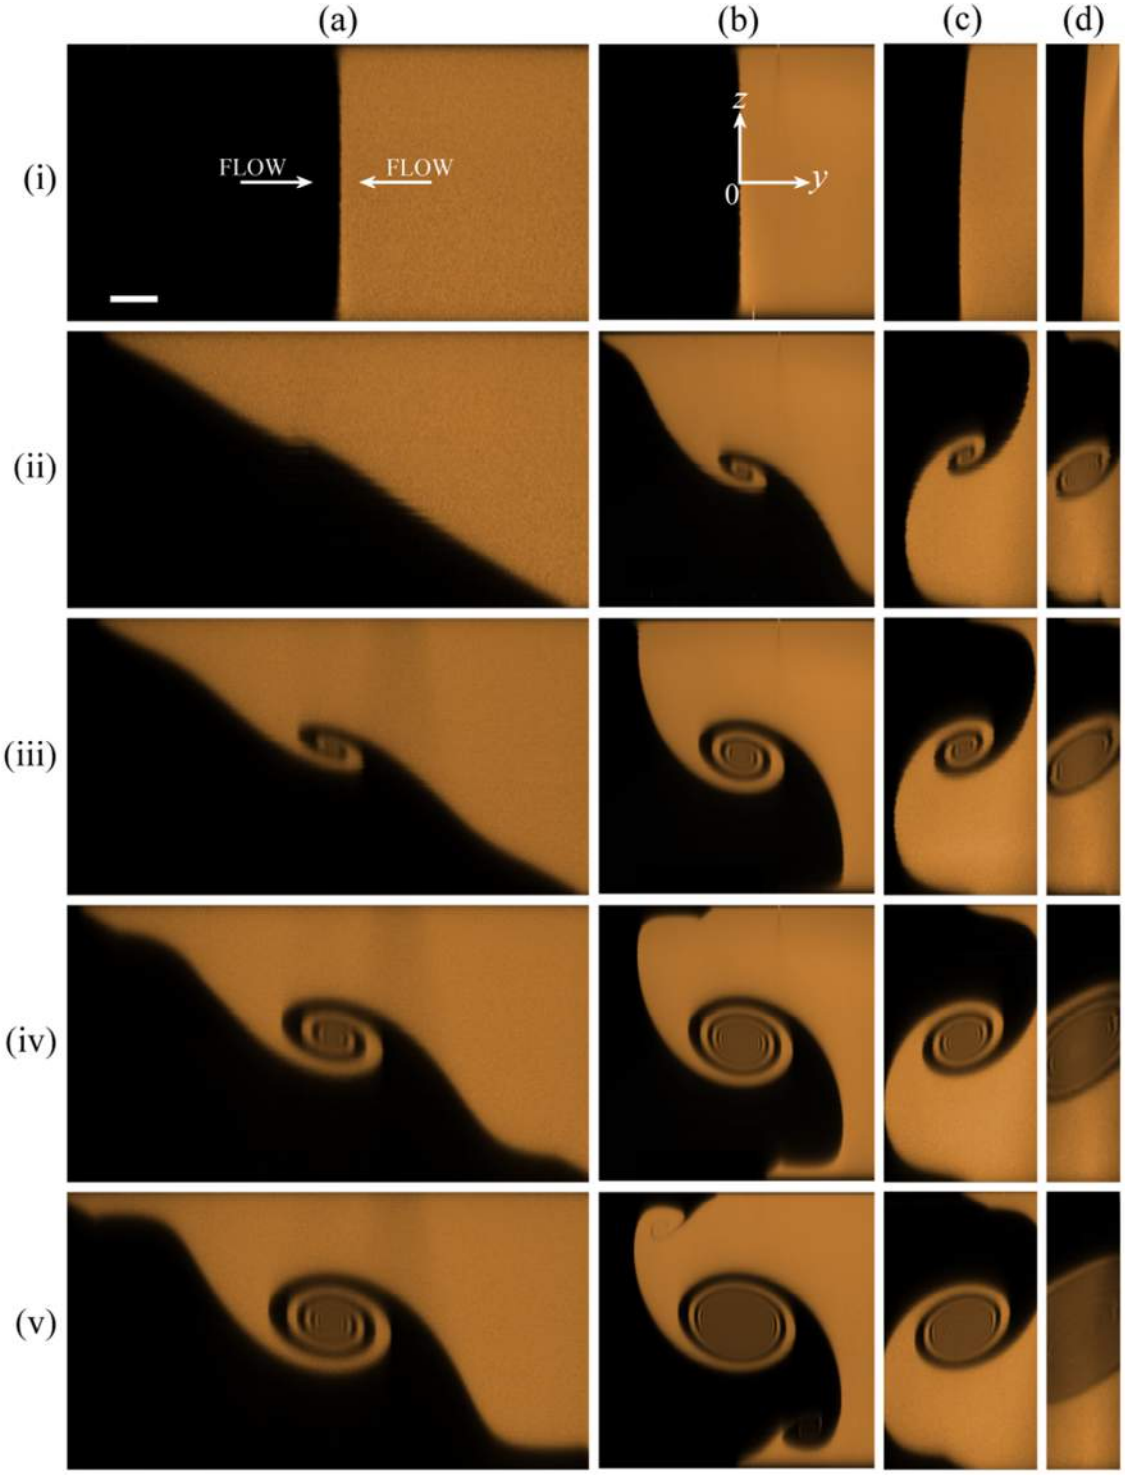


**FIG S2**: Confocal imaging depicting the evolution of flow structures in the $x = 0$ plane for Newtonian fluid flow in the various cross-slot devices under the following conditions:
(a) α = 0.49: (i) Re =30.3, (ii) Re = 100.1, (iii) Re = 104.6, (iv) Re = 121.3, (v) Re = 151.6.
(b) α = 1.00: (i) Re = 15.2, (ii) Re = 42.8, (iii) Re = 60.6, (iv) Re = 91.0, (v) Re = 151.6.
(c) α = 1.85: (i) Re = 7.6, (ii) Re = 23.5, (iii) Re = 26.5, (iv) Re = 33.4, (v) Re = 45.5.
(d) α = 3.87: (i) Re = 7.6, (ii) Re = 25.3, (iii) Re = 27.3, (iv) Re = 33.4, (v) Re = 45.5.
Fluorescently-dyed fluid enters from the right (positive $y$ ) and undyed fluid enters from the left (negative $y$ ); outflow is along $x$ (i.e. normal to the page). Images span $-w/2 \le y \le w/2$ , $-d/2 \le z \le d/2$ ; scale bar in (ai) represents 200 μm.

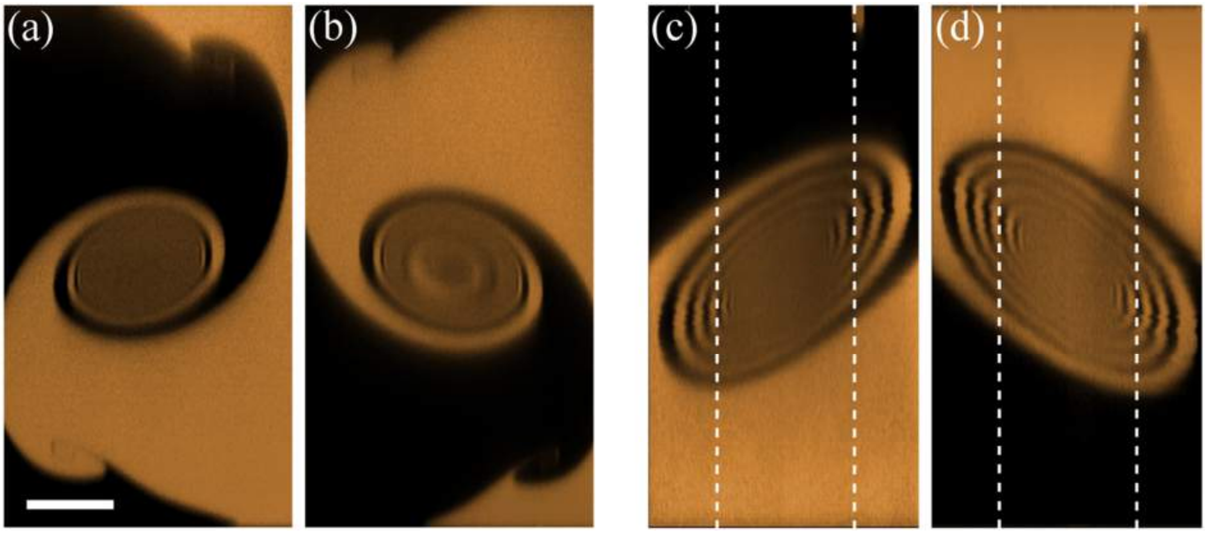


**FIG S3**: Examples of bi-handedness of the spiral vortex structure observed in the $x = 0$ plane: (a) and (b) flow in the cross-slot with α = 1.85 at Re = 66.7; (c) and (d) flow in the cross-slot with α = 3.87 at Re = 36.4. The scale bar in (a) represents 200 µm. The vertical dashed lines in (c) and (d) indicate the positions of the outlet channel corners at $y = \pm w/2$ . The two possible rotational orientations of the spiral correspond to positive and negative branches of the bifurcation. However, we only evaluate data obtained on one (favored) branch shown by parts (a) and (c) and which is considered positive.

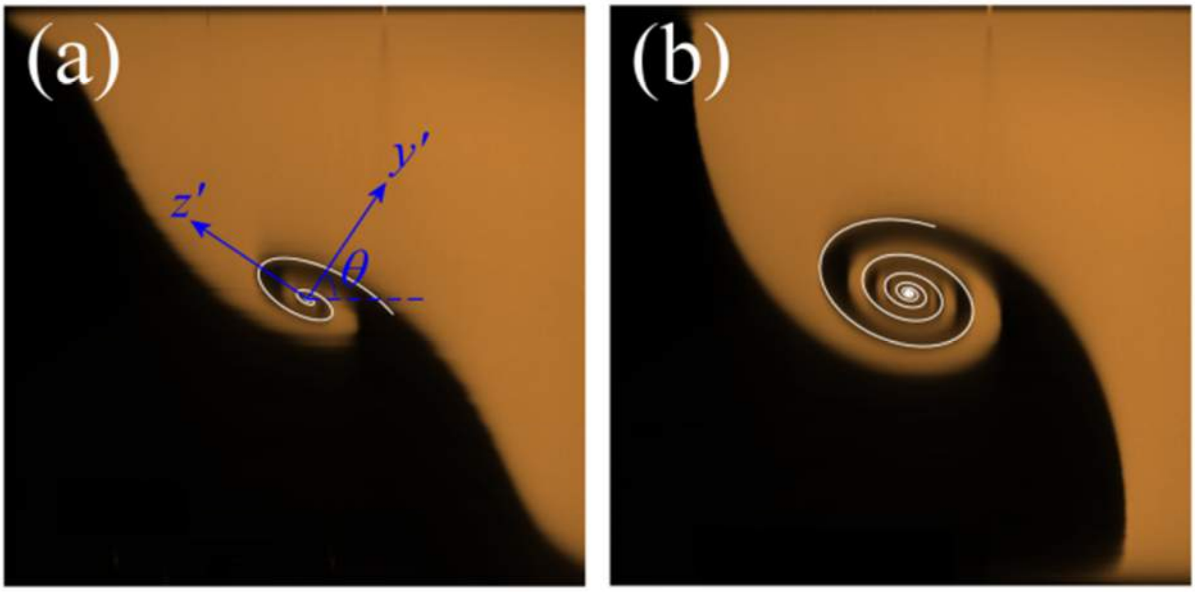


**FIG S4**: Images from the cross-slot (α = 1.00) superimposed with manually-fitted elliptical logarithmic spirals described parametrically as $y'(s) = a\cos(s)\,\mathrm{e}^{c/s}$, $z'(s) = b\cos(s)\,\mathrm{e}^{c/s}$ , where $(a-b)/a$ is the ellipticity and $c$ controls the rate of radial growth: (a) Re = 42.8,
(b) Re = 60.6.

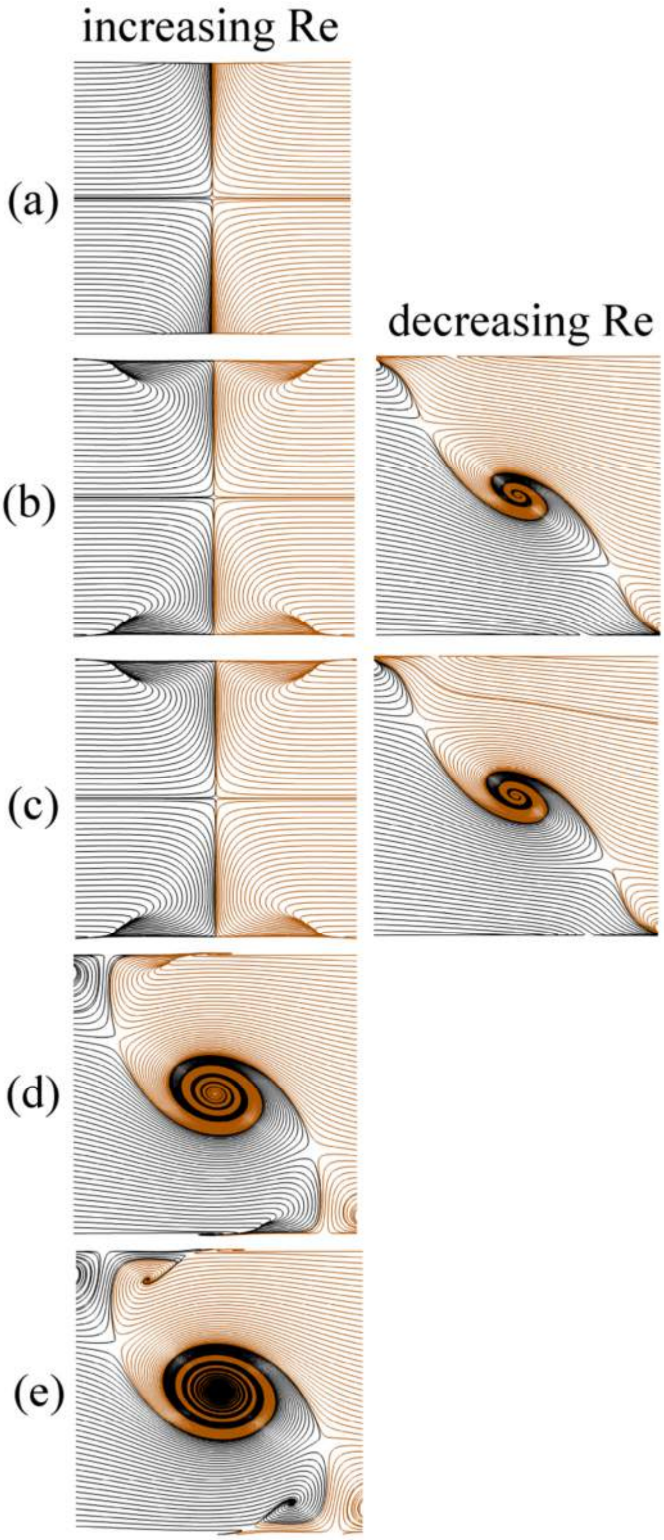


**FIG S5**: Numerically-determined streamlines depicting the evolution of flow structures in the $x = 0$ plane for Newtonian fluid flow in a cross-slot device with $\alpha = 1$ under the following conditions: (a) Re = 15.2 , (b) Re = 41.7 , (c) Re = 42.8, (d) Re = 60.6 , (e) Re = 91.0 . Hysteresis near the onset conditions results in two possible solutions for Re = 41.7 and Re = 42.8, depending on whether the Reynolds number is quasistatically increased or decreased.

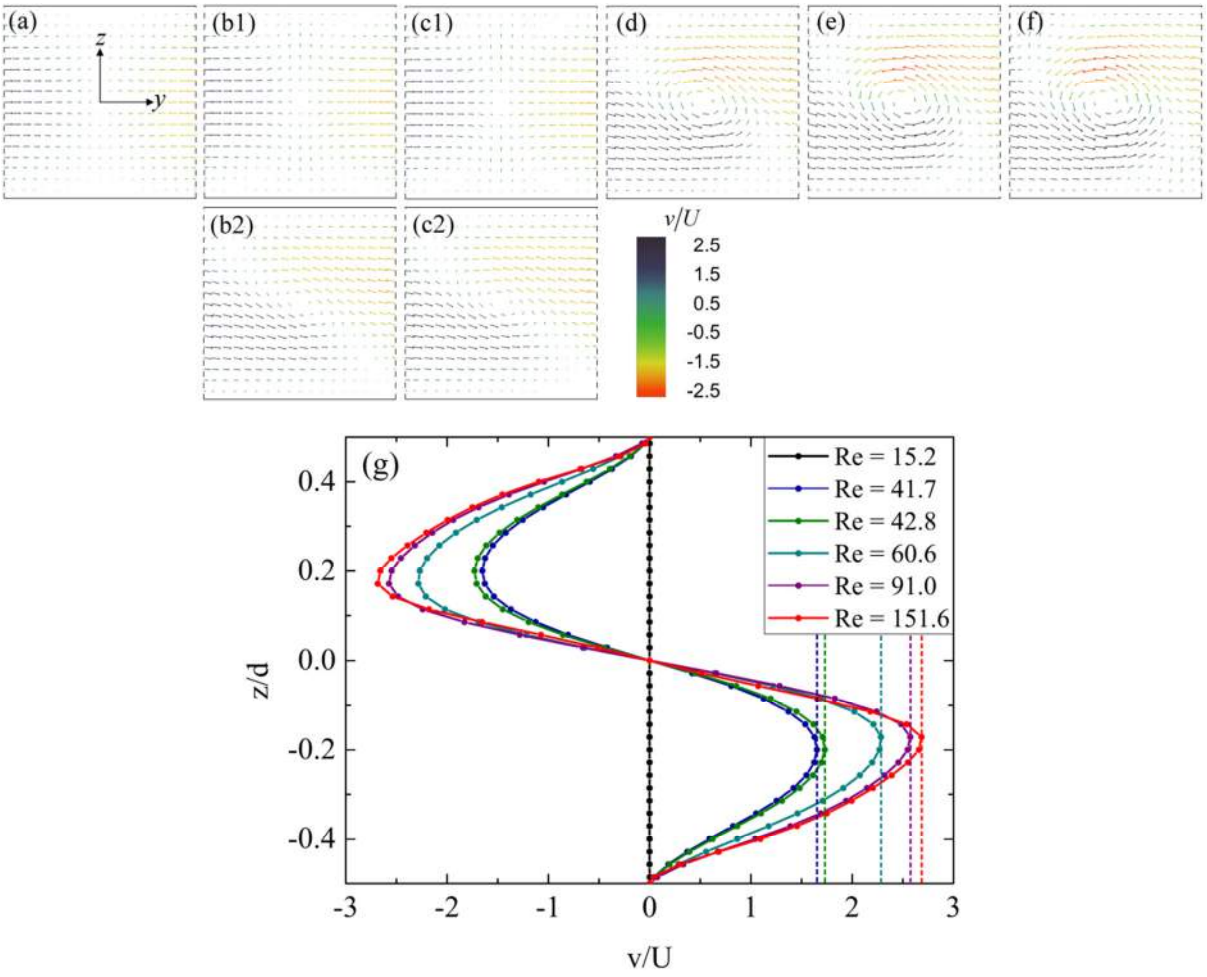


**FIG S6**: Numerically-determined vector velocity fields depicting the evolution of flow structures in the $x = 0$ plane for Newtonian fluid flow in a cross-slot device with $\alpha = 1$ under the following conditions: (a) Re = 15.2 , (b) Re = 41.7 , (c) Re = 42.8, (d) Re = 60.6 , (e) Re = 91.0 , (f) Re = 151.6 . For cases (b) and (c) both symmetric (1) and asymmetric (2) solutions are possible, depending on whether the Reynolds number is quasistatically increased or decreased, respectively. (g) Normalized $y$-velocity component measured along the $z$-axis (for quasistatic decreases in Re). The correspondingly colored vertical dashed lines indicate the value of the numerical order parameter, $M_{num} = v_{\max}\big|_{x=y=0} \big/ U$ measured at each Re.

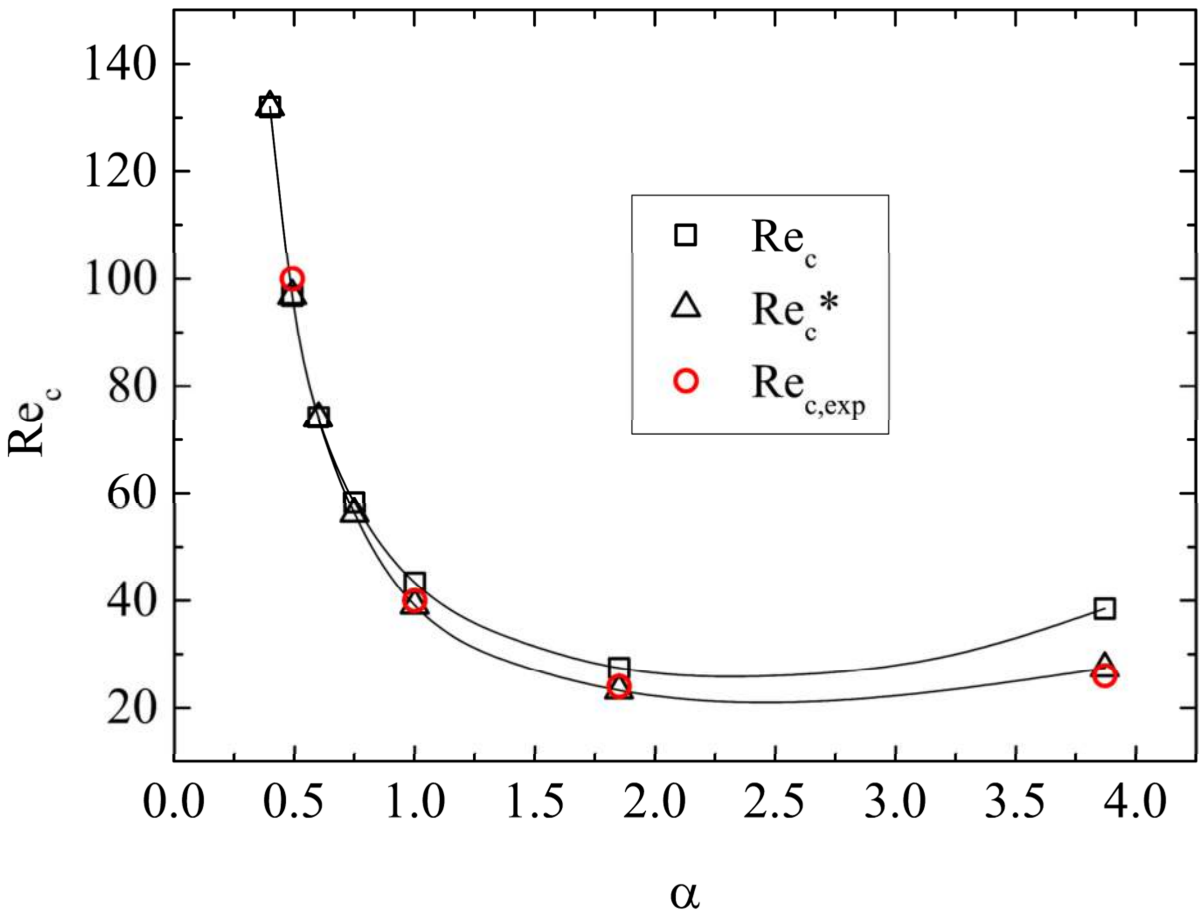


**FIG S7**: Comparison between experimental and numerical critical Reynolds numbers for flow in cross-slot devices with various aspect ratios. $Re_c$ is the critical Re determined from numerical simulations for quasistatic increases in Re. $Re_c$* is the critical Re determined from numerical simulations for quasistatic decreases in Re. For forward bifurcations $Re_c = Re_c$*, however for backward bifurcations, hysteresis in the transition onset means $Re_c^* < Re_c$. The apparent critical Reynolds number from the experiment, $Re_{c,exp}$ agrees well with $Re_c$*.
